# Supplementary material for: XAttention: Block Sparse Attention with Antidiagonal Scoring
Source: arXiv:2503.16428 source file (2025-03-20)
Supplement: Supplementary file 1 [file appendix.tex]

\newpage
\appendix
\onecolumn
\section{A. Math Proof}

\textbf{Rule 1 (Information Preservation):} To retain all token information, for an \(n \times n\) attention block, we must select at least one element from each row and each column.  To minimize computational cost, we aim to select precisely \(n\) tokens in the ideal case.

\textbf{Rule 2 (Pattern Similarity):}  We aim to select blocks such that the sum of the selected patterns and the full attention map demonstrate high similarity, both in terms of the order of their sums and the distribution of the summed values. We quantify this similarity using two metrics:

\begin{itemize}
    \item \textbf{Order Similarity:} Measured by the correlation of the ranks of the sums.
    $$
    \text{Similarity}_{\text{order}} = \text{Corr}( \text{rank}(S_{\text{selected}}), \text{rank}(S_{\text{full}}) )
    $$
    \item \textbf{Distribution Similarity:} Measured by the Jensen-Shannon divergence between the probability distributions.
    $$
    \text{Similarity}_{\text{distribution}} = D_{\text{JS}}( P_{\text{selected}} \parallel P_{\text{full}} )
    $$
\end{itemize}

Here, \(S_{\text{selected}}\) and \(S_{\text{full}}\) represent the sums of the selected elements and the full attention map, respectively. \(P_{\text{selected}}\) and \(P_{\text{full}}\) are their corresponding probability distributions.

To achieve this, we propose the \textbf{antidiagonal scoring pattern} for \method. We observe that selecting elements along the antidiagonal, defined as:
$$
A_{i,j} = q_{n-i-1} \cdot k_{i}, \quad \text{for } i \in [0, n-1]
$$
can effectively approximate the full attention sum:
$$
S_{\text{full}} = \sum_{i=0}^{n-1} \sum_{j=0}^{n-1} q_i \cdot k_j
$$
where \(q_i\) represents the query vector and \(k_i\) represents the key vector at position \(i\).

%%%%%%%%%%%%%%%%%%%%%%%%%%%%%%%%%%%%%%%%%%%%%%%%%%%%%%%%%%%%%%%%%%%%%%%%%%%%%%%
%%%%%%%%%%%%%%%%%%%%%%%%%%%%%%%%%%%%%%%%%%%%%%%%%%%%%%%%%%%%%%%%%%%%%%%%%%%%%%%
